# Supplementary material for: Sion's Minimax Theorem in Geodesic Metric Spaces and a Riemannian Extragradient Algorithm
Source: arXiv:2202.06950 source file (2023-05-29)
Supplement: Supplementary file 1 [file sec_8_suppl.tex]

\section{Supplementary} \label{sec: suppl}
In this supplementary section, we provide some related background and technical details.

%\subsection{Curvature and comparison inequalities} \label{appendix: complete}

\paragraph{Strongly convex function in metric space} We first provide a definition of strong convexity in geodesic metric space, of which we omit in the previous sections. Note that the definition subsumes the regularity definition of strongly convex function in Riemannian optimization.
\begin{definition} [Strong convexity] \label{def: g-sc}
     Suppose $\mfld$ is a geodesic metric space. A function $f: \mfld \rightarrow \bbR$ is geodesically strongly-convex modulus $\mu$, if, for any $x, y \in \mfld$ and $t \in [0,1]$, following inequality holds: $f(\gamma(t)) \leq tf(x) + (1 - t)f(y) + \tfrac{\mu t(1-t)}{2} d_{\mfld}^2(x, y)$, where $\gamma$ is the geodesic connecting $x,y$.
\end{definition}
\begin{remark}
$f$ is geodesically strongly-concave modulus $\mu$ if $-f$ is geodesically $\mu$-strongly-convex.
\end{remark}
%\paragraph{Unique and complete geodesic structure}
